# Supplementary material for: RL-ScanIQA: Reinforcement-Learned Scanpaths for Blind 360{\deg}Image Quality Assessment
Source: arXiv:2603.14297 source file (2026-03-15)
Supplement: Supplementary file 1 [file X_suppl.tex]

\clearpage
\setcounter{page}{1}
\maketitlesupplementary

In this supplementary material, we extend more ablation studies in Section A and implementation details about distortion-space augmentation in Section B. Furthermore, we also show more visualizations about augmentation and generated scanpaths in Section C. 

\section*{A. More Ablation Studies}
\label{sec:abl}
\noindent\textbf{Impact of Shannon Entropy Step-Wise Reward.} To explore how Shannon Entropy reward contributes to the policy learning, we remove the Shannon Entropy reward $\mathcal{H}(x_t)$ in step-wise exploration rewards, referred to as (\emph{w/o $\mathcal{H}(x_t)$}), while keeping all other components unchanged. As shown in Table \ref{tab:each reward}, removing the entropy cue has the largest effect on scenarios featuring non‑uniform degradations. This indicates that entropy‑guided exploration steers the policy toward structurally informative regions and mitigates undersampling of quality‑critical content.

\vspace{3pt}\noindent\textbf{Impact of Dissimilarity-Based Step-Wise Reward.}
To explore how the dissimilarity reward contributes to the RL policy learning, we remove the term $1 - \text{SSIM}(x_{t-1}, x_t)$ in step-wise rewards, denoted as (\emph{w/o $1 - \text{SSIM}(x_{t-1}, x_t)$}), while keeping all other settings unchanged. As shown in Table \ref{tab:each reward}, removing the dissimilarity cue leads to large drops on JUFE, moderate on OIQA, and smallest on CVIQD, reflecting the datasets’ increasing spatial uniformity. This pattern indicates that the term $1 - \mathrm{SSIM}(x_{t-1}, x_t)$ is critical for suppressing near-duplicate transitions, broadening spherical coverage within a scanpath, and exposing localized degradations that better align exploration with the IQA objective.

\vspace{3pt}\noindent\textbf{Impact of Novelty Signal Step-Wise Reward.}
To explore how the novelty signal reward contributes to the RL policy learning, we remove the novelty signal $\delta_\text{new}(x_t)$ in step-wise rewards, referred to as (\emph{w/o $\delta_\text{new}(x_t)$}), while keeping all other settings unchanged. As shown in Table \ref{tab:each reward}, the results confirm that the novelty signal helps break local loops and surface localized artifacts under non‑uniform degradations.

\vspace{3pt}\noindent\textbf{Impact of Equator-Bias Prior Step-Wise Reward.}
To explore how equator-bias prior contributes to the RL policy learning, we remove equator-bias prior $\mathcal{B}(x_t)$ in step-wise rewards, referred to as (\emph{w/o $\mathcal{B}(x_t)$}), while keeping all other settings unchanged. As shown in Table \ref{tab:each reward}, removing the equator-bias prior leads to the mildest degradation among all step-wise cues. This pattern suggests that \(\mathcal{B}(x_t)\) mainly serves as a soft, human-consistent prior that stabilizes exploration toward informative equatorial regions—useful under spatially non-uniform degradations but not the primary driver of coverage or redundancy reduction.

\noindent\textbf{Impact of Similarity Consistency Loss.}
To explore the contribution of similarity consistency to cross-dataset generalization, we remove the similarity consistency loss, referred to as (\emph{w/o $\mathcal{L}_\text{cons}$}), while keeping all others unchanged. As shown in Table \ref{tab:each loss}, removing $\mathcal{L}_\text{cons}$ results in calibration (PLCC) drops larger than ranking (SRCC). This matches its role in enforcing prediction smoothness under weak perturbations and improving cross‑domain score calibrations.

\noindent\textbf{Impact of Triplet Loss.}
To explore the effectiveness of triplet loss on cross-dataset generalization, we remove the triplet loss, while keeping all others unchanged, referred to as (\emph{w/o $\mathcal{L}_\text{triplet}$}). As shown in Table \ref{tab:each loss}, the result matches its role in enforcing the clean–mild–strong severity ordering, which primarily stabilizes cross‑domain score calibration rather than inter‑image ranking.

\noindent\textbf{Impact of Cross-Rank Loss.}
To explore how the cross-rank loss contribute to the cross-dataset generalization, we remove the cross-rank loss, while keeping all others unchanged, refereed to as (\emph{w/o $\mathcal{L}_\text{cross}$}). As shown in Table \ref{tab:each loss}, removing cross-rank loss $\mathcal{L}_\text{cross}$ causes the largest SRCC drops among all loss ablations. This matches its role in preserving inter‑image orders after augmentation and complements $\mathcal{L}_\text{cons}$ and $\mathcal{L}_\text{triplet}$.

\setlength{\tabcolsep}{1mm}
\begin{table}
\centering
\caption{Ablation study on multiple rewards.}
\vspace{-3mm}
\label{tab:each reward}
\resizebox{\columnwidth}{!}{
\begin{tabular}{lcccccc}
\toprule
\multirow{2}{*}{\textbf{Method}} & \multicolumn{2}{c}{\textbf{CVIQD}} & \multicolumn{2}{c}{\textbf{OIQA}} & \multicolumn{2}{c}{\textbf{JUFE}} \\
\cmidrule(lr){2-3} \cmidrule(lr){4-5} \cmidrule(lr){6-7}
& \textbf{SRCC} & \textbf{PLCC} & \textbf{SRCC} & \textbf{PLCC} & \textbf{SRCC} & \textbf{PLCC} \\
\midrule
w/o $\mathcal{H}(x_t)$ & 0.963 & 0.968 & 0.935 & 0.963 & 0.801 & 0.872 \\
w/o $1 - \text{SSIM}(x_{t-1}, x_t)$ & 0.958 & 0.963 & 0.931 & 0.956 & 0.791 & 0.852 \\
w/o $\delta_\text{new}(x_t)$ & 0.955 & 0.962 & 0.933 & 0.960 & 0.796 & 0.862 \\
w/o $\mathcal{B}(x_t)$ & 0.967 & 0.973 & 0.938 & 0.965 & 0.808 & 0.886 \\
\textbf{Main Model} & \textbf{0.968} & \textbf{0.977} & \textbf{0.941} & \textbf{0.967}& \textbf{0.816} & \textbf{0.902} \\
\bottomrule
\vspace{-4mm}
\end{tabular}
}
\end{table}

\setlength{\tabcolsep}{0.5mm}
\begin{table}[t]
	\centering
	\footnotesize
    \caption{Ablation study on multiple losses.}
    \vspace{-7mm}
	\begin{center}
		{
        \resizebox{1.0\columnwidth}{!}
		{
			\begin{tabular}{l | cc | cc}
						\toprule
						\multirow{2}{*}{\textbf{Method}} 
& \multicolumn{2}{c|}{\makecell{Train: \textbf{CVIQD} \\ Test: \textbf{OIQA} / \textbf{JUFE}}} 
& \multicolumn{2}{c}{\makecell{Train: \textbf{JUFE} \\ Test: \textbf{CVIQD} / \textbf{OIQA}}} \\ 
\cline{2-5}
& \textbf{SRCC} & \textbf{PLCC} & \textbf{SRCC} & \textbf{PLCC} \\ 
\hline
w/o $\mathcal{L}_\text{cons}$
& 0.877/ 0.794 & 0.894 / 0.787
& 0.739 / 0.740 & 0.762 / 0.765\\
w/o $\mathcal{L}_\text{triplet}$
& 0.860 / 0.792 & 0.872 / 0.760 
& 0.729 / 0.732 & 0.746 / 0.698\\
w/o $\mathcal{L}_\text{cross}$
& 0.847 / 0.789 & 0.884 / 0.801 
& 0.708 / 0.712 & 0.745 / 0.771\\
\textbf{Main Model} 
& \textbf{0.901} / \textbf{0.800} & \textbf{0.913} / \textbf{0.822} 
& \textbf{0.771} / \textbf{0.755} & \textbf{0.802} / \textbf{0.833} \\				
						\bottomrule
						
				\end{tabular}
		}}
	\end{center}
    \label{tab:each loss}
    \vspace{-3mm}
\end{table}

\section*{B. Distortion-Space Augmentation Details}
\label{sec:aug}

\begin{figure*}
\includegraphics[width=\textwidth]{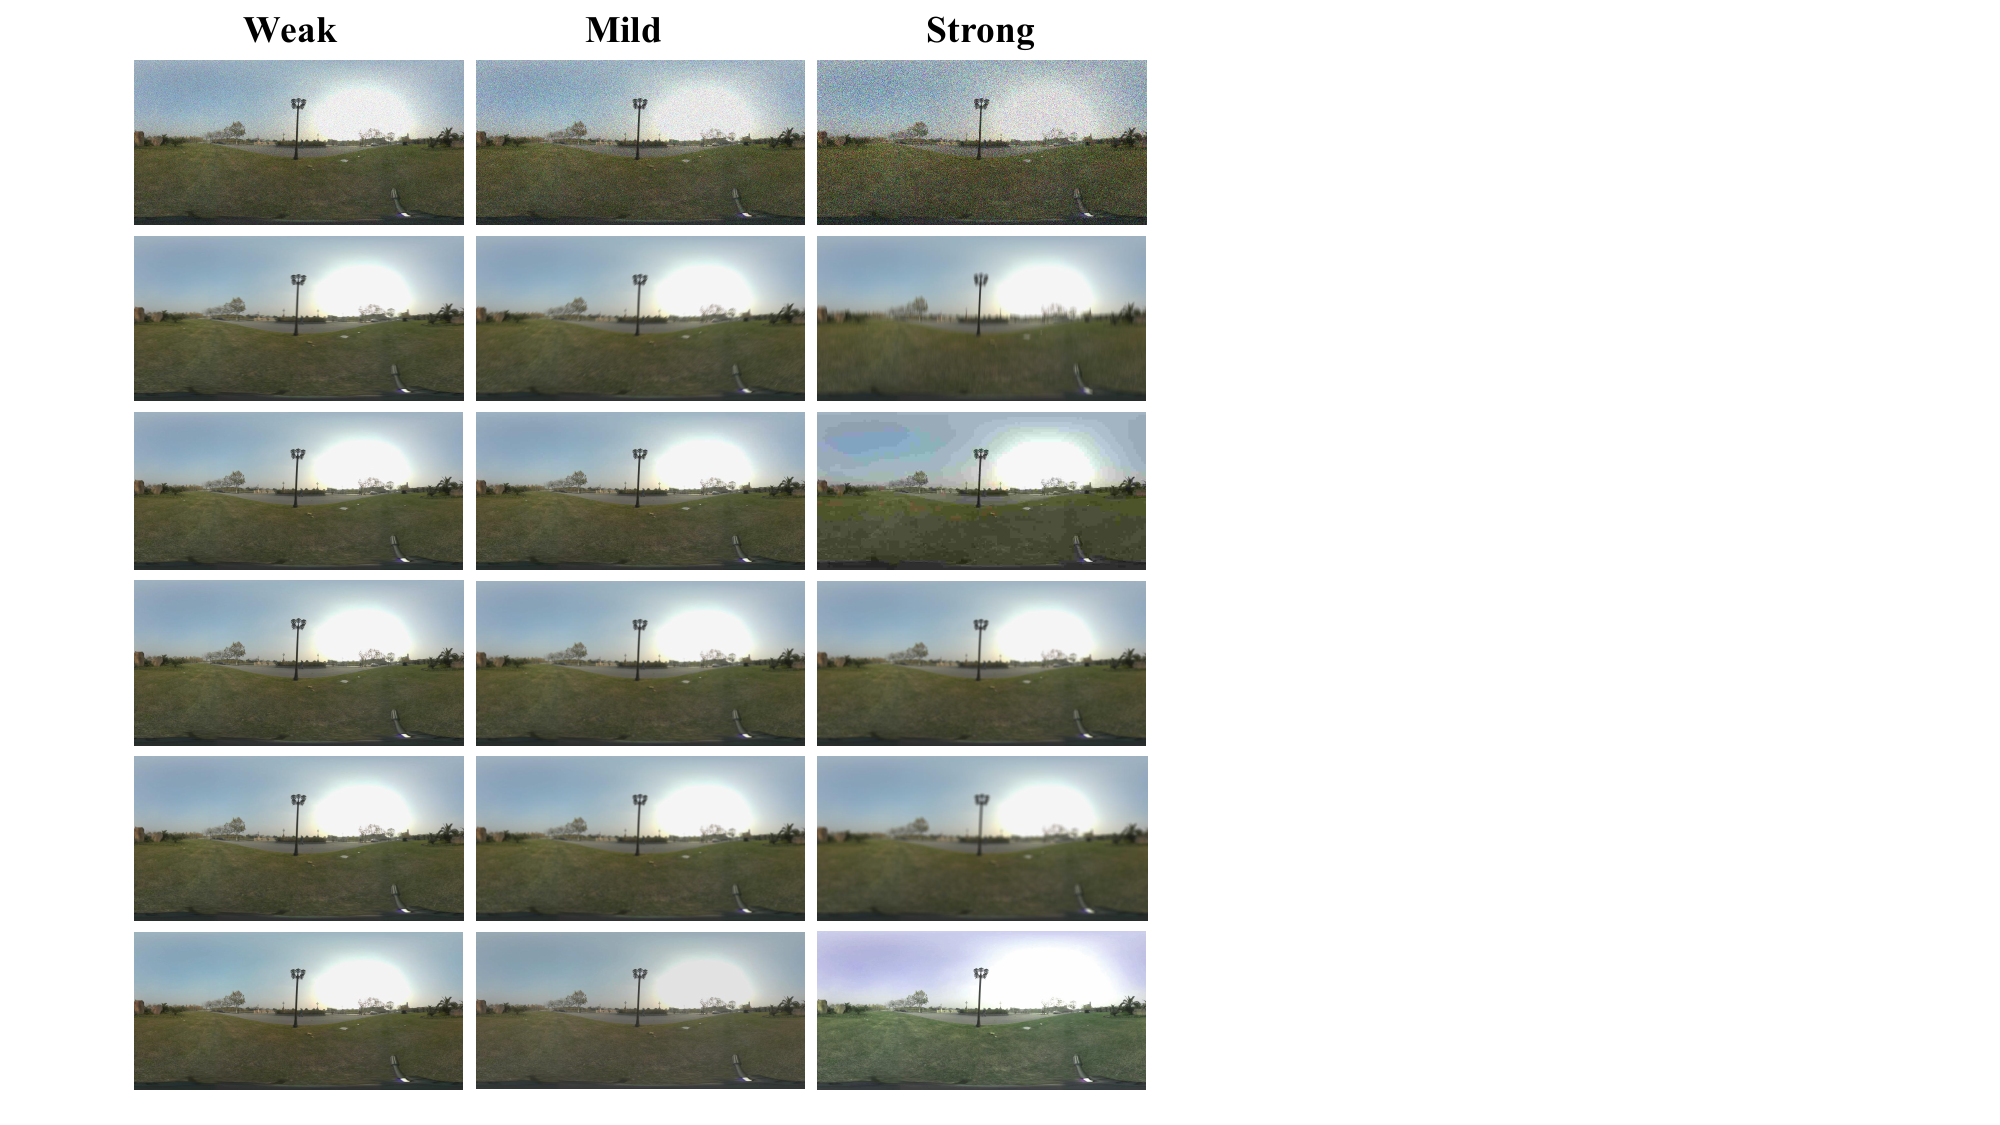}
\vspace{-6mm}
  \caption{Distortion-space augmented images with different severity levels. From left to right, images are appended by weak, mild, and strong augmentations, respectively.
  }
  \vspace{-4mm}
  \label{aug}
\end{figure*}

To enhance cross-domain robustness, we apply a set of distortion-space augmentations that simulate diverse real-world degradations. Following our main paper, each input image is augmented into three severity levels: weak, mild, and strong, with increasing perceptual distortion. Specifically, weak augmentations are randomly sampled from compression, blur, or color jitter, consistent with the Similarity Consistency Loss design. In contrast, mild and strong augmentations are drawn from a broader space that includes JPEG compression, motion blur, defocus blur, color jitter, and Poisson noise.

\begin{figure*}
\includegraphics[width=\textwidth]{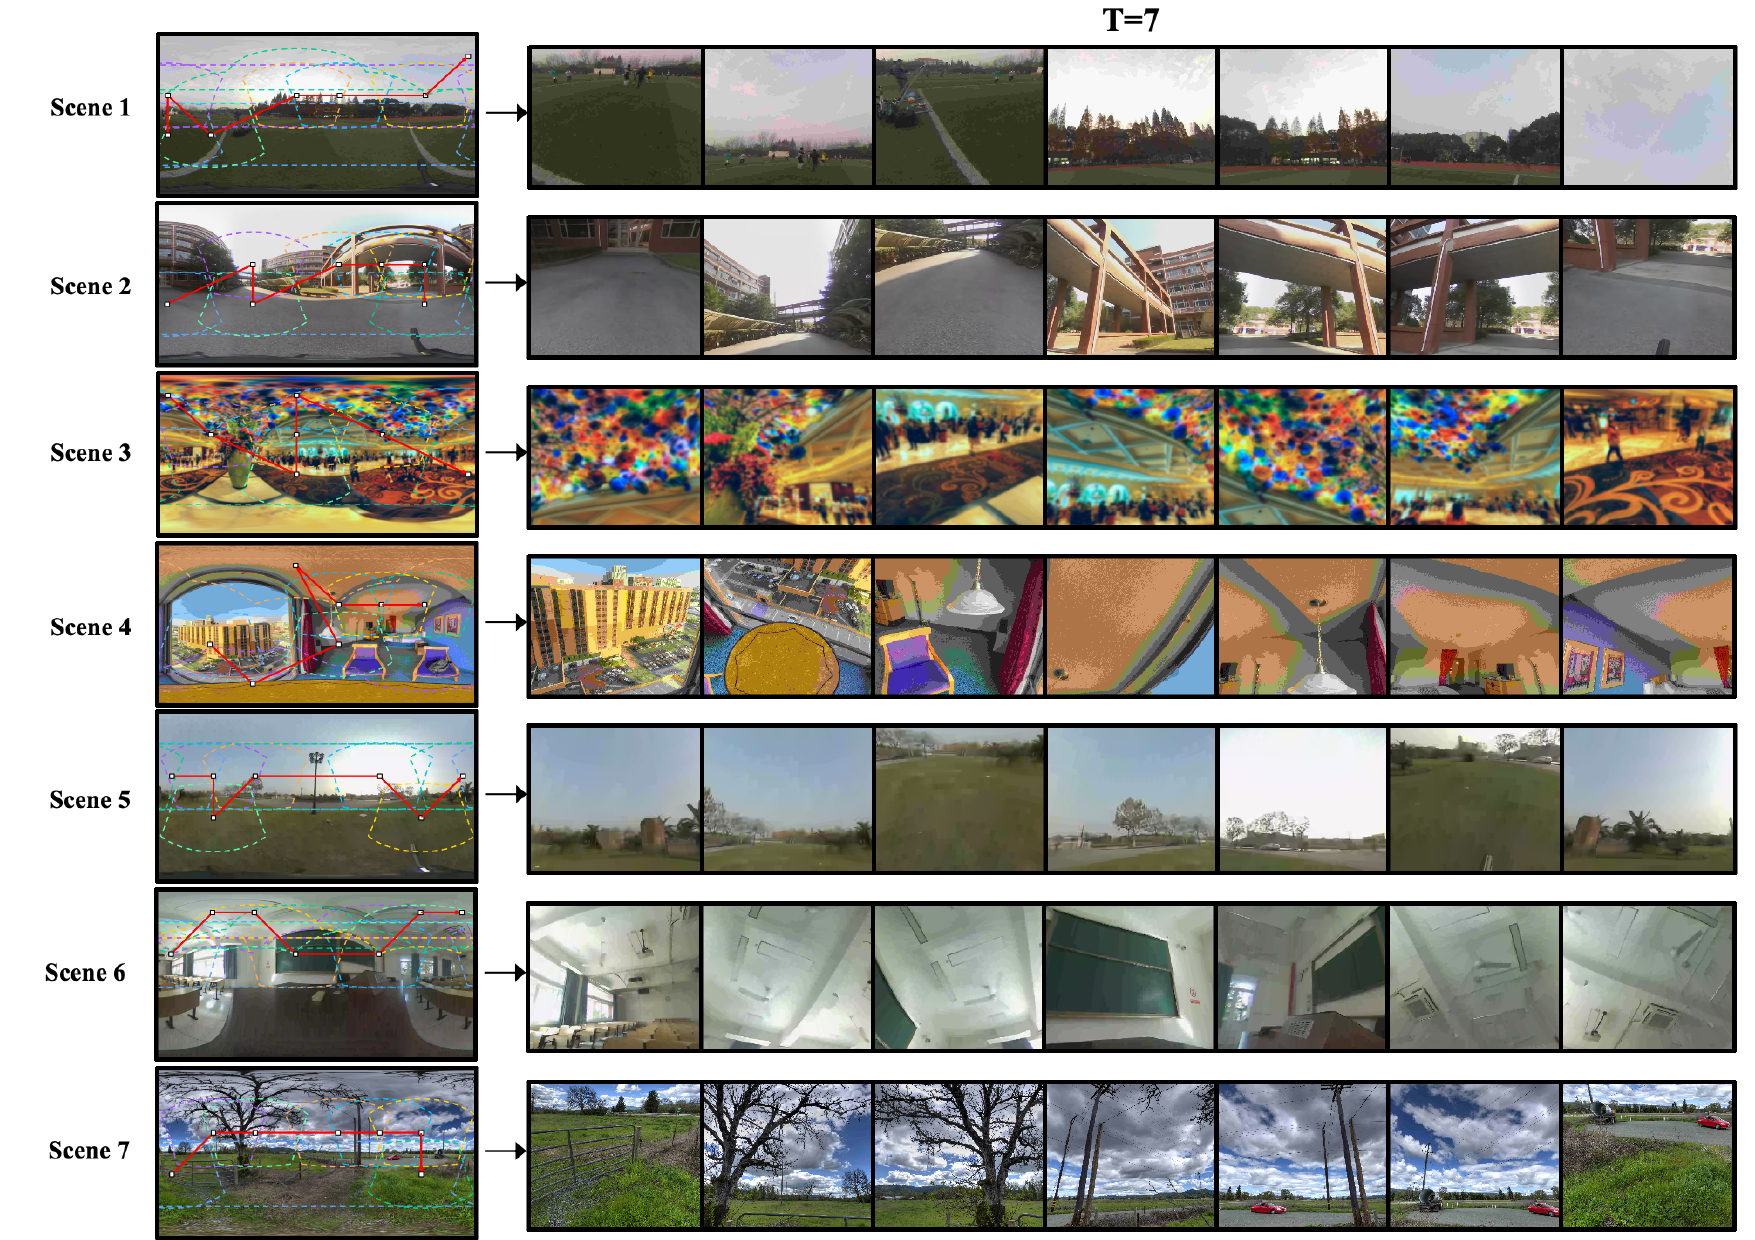}
\vspace{-6mm}
  \caption{Visualization of generated scanpath and viewports. 
  }
  \vspace{-4mm}
  \label{scan}
\end{figure*}

JPEG compression quality is set to $q\in[85,95]/[60,75]/[20,40]$ for weak/mild/strong, respectively; motion blur uses kernel lengths of $k\in[3,7]/[7,11]/[11,19]$ with random angle; defocus blur adopts disk radii $r\in[1,2]/[2,3]/[4,6]$; color jitter scales brightness, contrast, saturation, and hue with increasing magnitude; Poisson noise is applied with $\lambda\in[18,30]/[6,12]$. Each augmented version is produced by sampling one distortion type and one parameter setting per level, without composing multiple distortions. These augmentations are used to supervise three loss terms during training: (i) Similarity Consistency (clean vs. weak), (ii) Triplet Ranking (clean, mild, strong), and (iii) Cross-Rank Consistency (across images under mild/strong augmentations). Visualization examples of these augmentations are provided in Figure \ref{aug}.

\section*{C. More Learned Scanpath Visualization}
In Figure \ref{scan}, we visualize seven scenes with one generated scanpath and corresponding viewports for each scene. Our policy-learned scanpaths can effectively capture severely distorted regions in the image, which is important for image perceptual quality assessment. For example, in Scene 2, the viewports in T=2,3,6 and 7, effectively capture the distortion regions. In Scene 3, the dominant factor degrading perceptual quality is the strong blur in the upper region. Our policy‑learned scanpath naturally focuses on this heavily distorted area, which is crucial for the accurate quality assessment.

%To split the supplementary pages from the main paper, you can use \href{https://support.apple.com/en-ca/guide/preview/prvw11793/mac#:~:text=Delete%20a%20page%20from%20a,or%20choose%20Edit%20%3E%20Delete).}{Preview (on macOS)}, \href{https://www.adobe.com/acrobat/how-to/delete-pages-from-pdf.html#:~:text=Choose%20%E2%80%9CTools%E2%80%9D%20%3E%20%E2%80%9COrganize,or%20pages%20from%20the%20file.}{Adobe Acrobat} (on all OSs), as well as \href{https://superuser.com/questions/517986/is-it-possible-to-delete-some-pages-of-a-pdf-document}{command line tools}.
